# Supplementary material for: Electrical-equivalent van der Waals gap for 2D bilayers
Source: arXiv:1803.10009 source file (2018-03-27)
Supplement: Supplementary file 1 [file Supplementary_material.pdf]

# Electrical-equivalent van der Waals gap for 2D bilayers
## Supplemetary Material

Figures S1, S3, S5, S7, S9 (S2, S4, S6, S8, S10) show the comparison of electrostatic model without tail length correction ( with electrical tail length correction) and density functional theory simulations in calculating the  band alignments of top and bottom MLs in a TMD bilayer system. In each figure subfigure (a) is for the interlayer separation (chalcogen to chalcogen distance) of 4 Å, subfigure (b) is for  5 Å, subfigure (c) is for 6 Å and subfigure is for 7 Å. The disagreement in the electrostatic model and DFT approach can be easily observed.

**Figure S1: $MoS_2$ BL system – uncorrected electrostatic model**

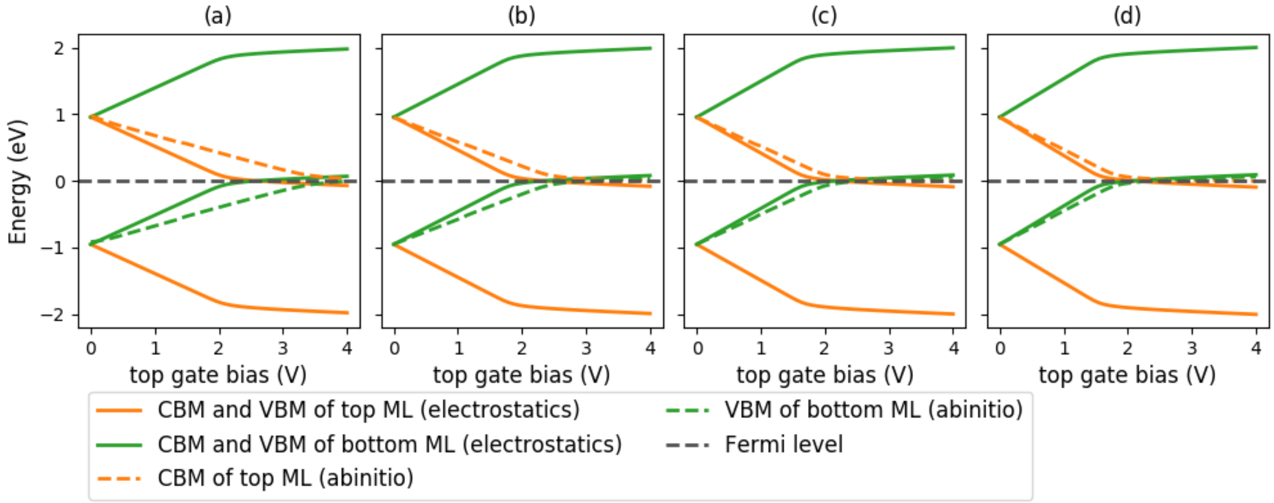


**Figure S2: $MoS_2$ BL system – tail length corrected electrostatic model**

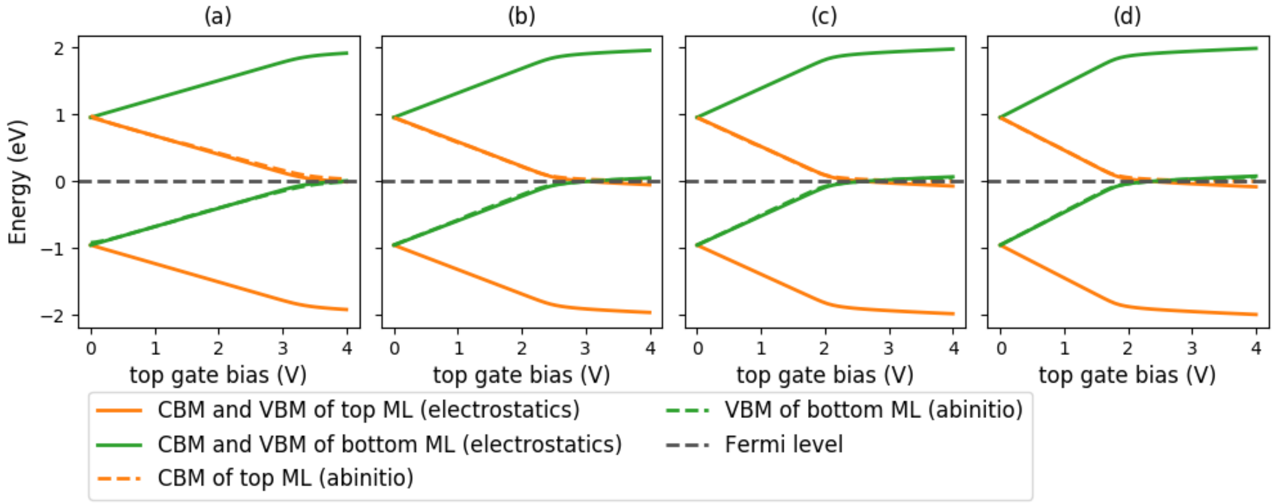

**Figure S3: $MoSe_2$ BL system – uncorrected electrostatic model**

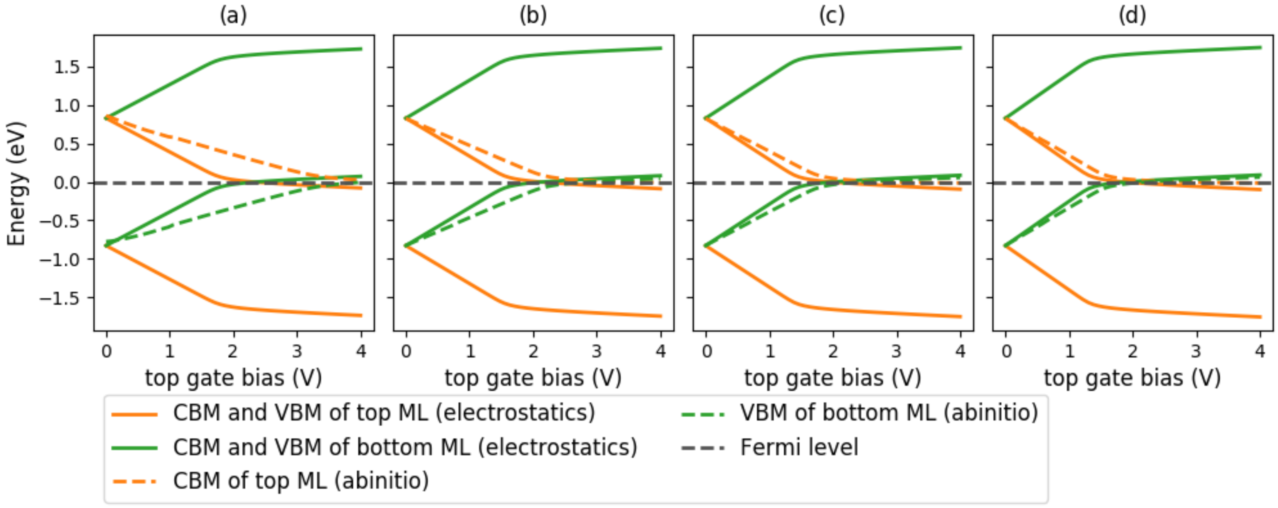


**Figure S4: $MoSe_2$ BL system – tail length corrected electrostatic model**

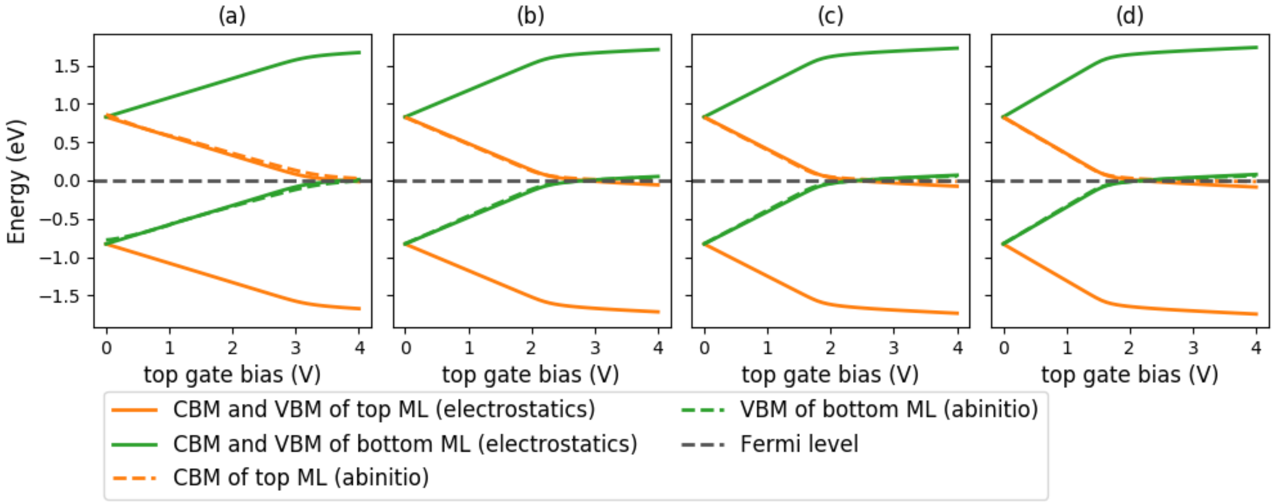

**Figure S5: $MoTe_2$ BL system – uncorrected electrostatic model**

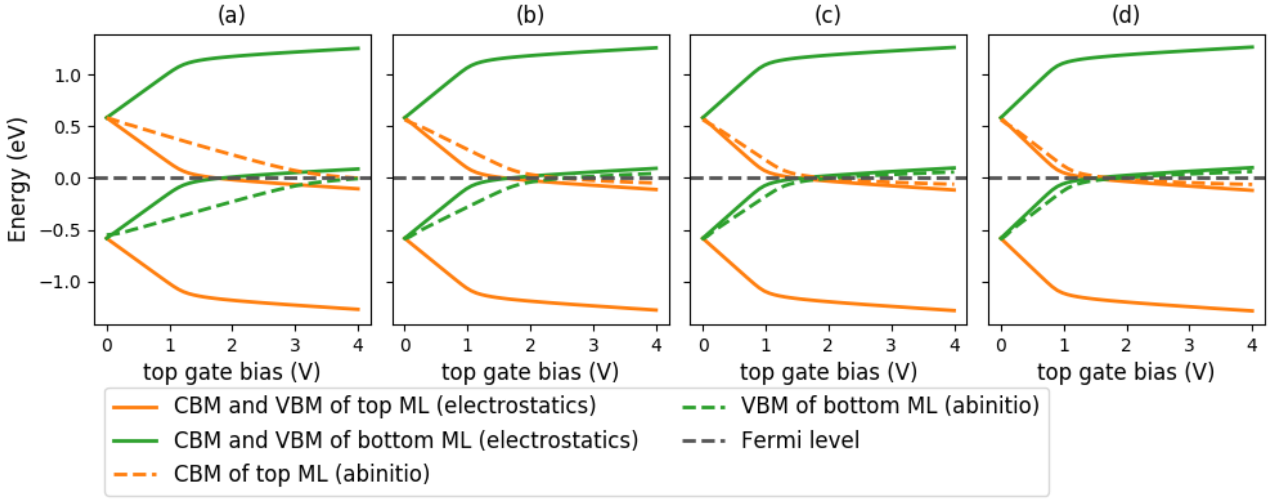


**Figure S6: $MoTe_2$ BL system – tail length corrected electrostatic model**

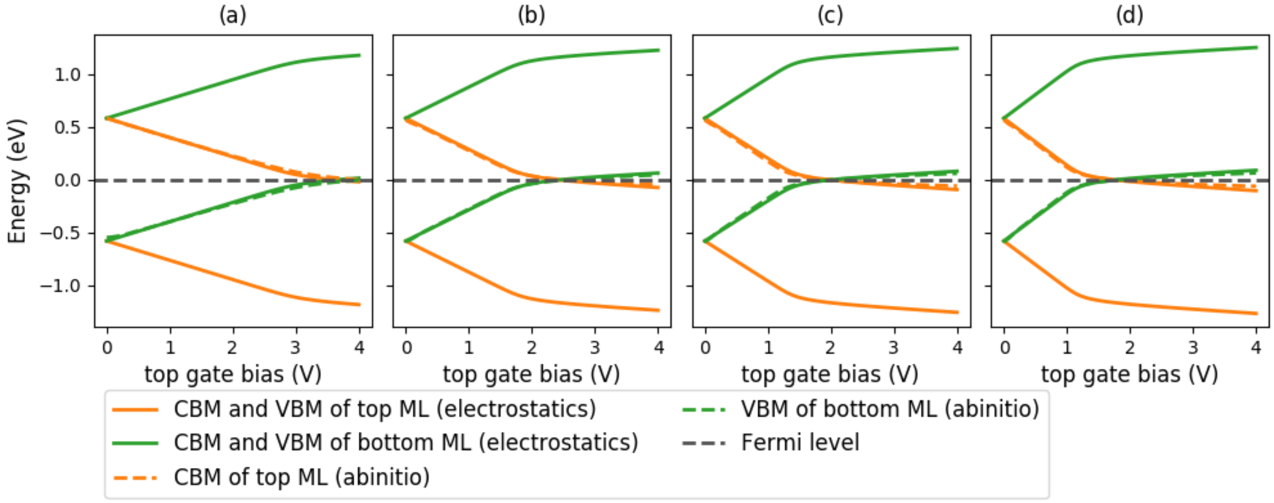

**Figure S7: $WSe_2$ BL system – uncorrected electrostatic model**

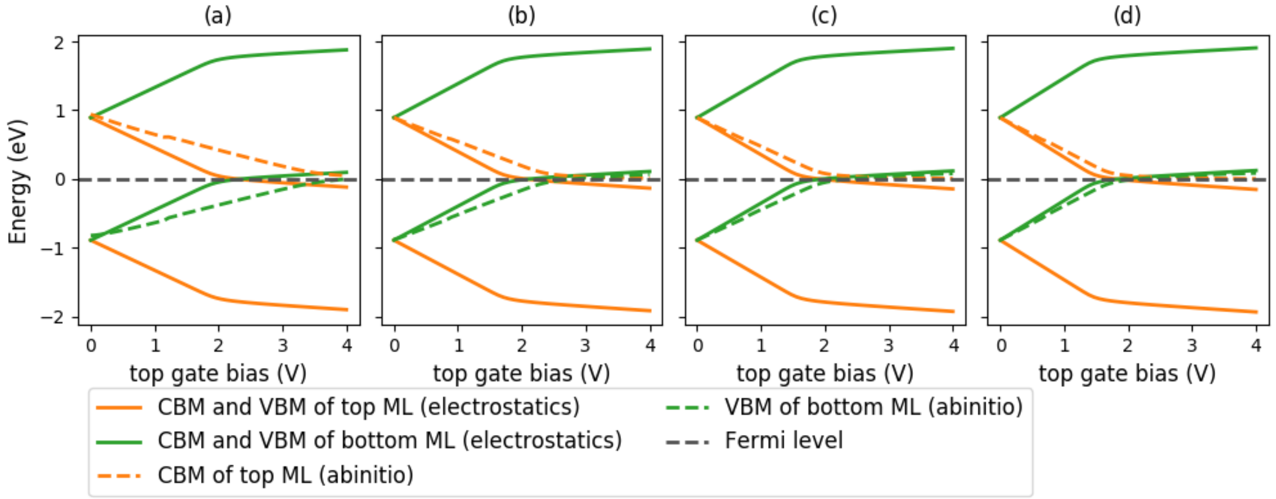


**Figure S8: $WSe_2$ BL system – tail length corrected electrostatic model**

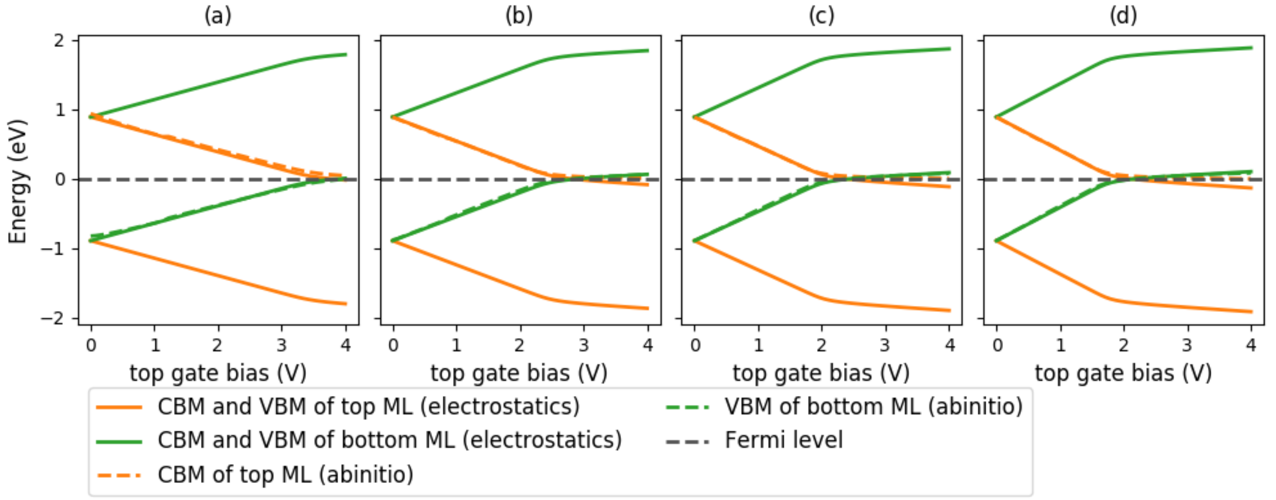

**Figure S9: $WTe_2$ BL system – uncorrected electrostatic model**

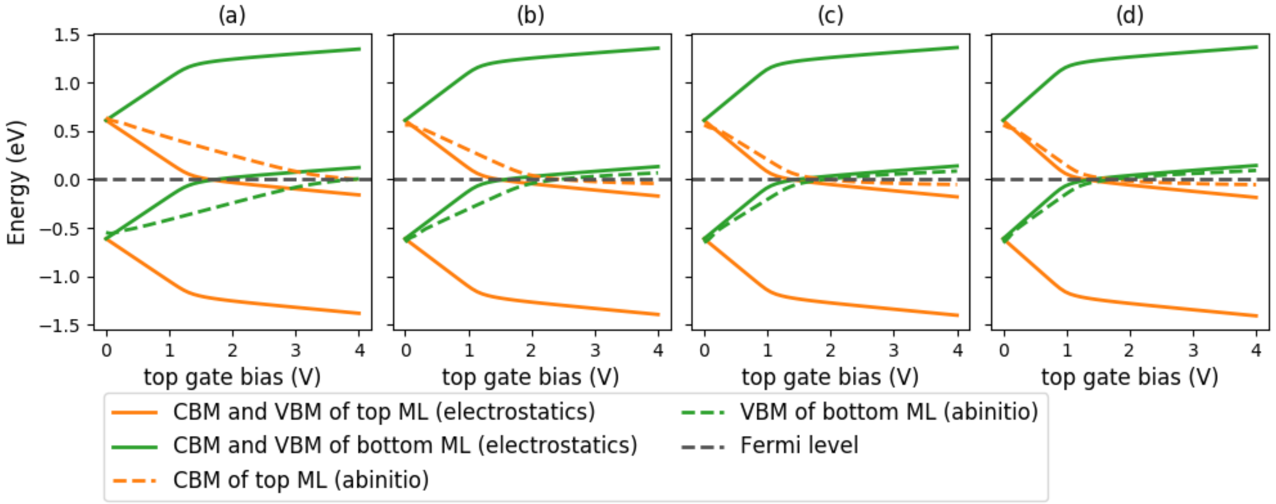


**Figure S10: $WTe_2$ BL system – tail length corrected electrostatic model**

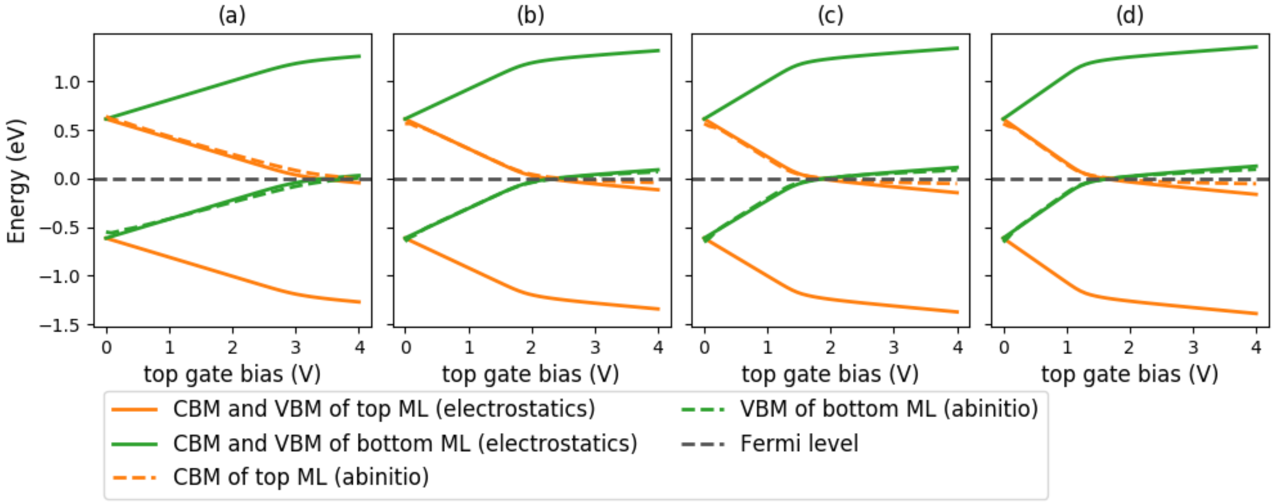

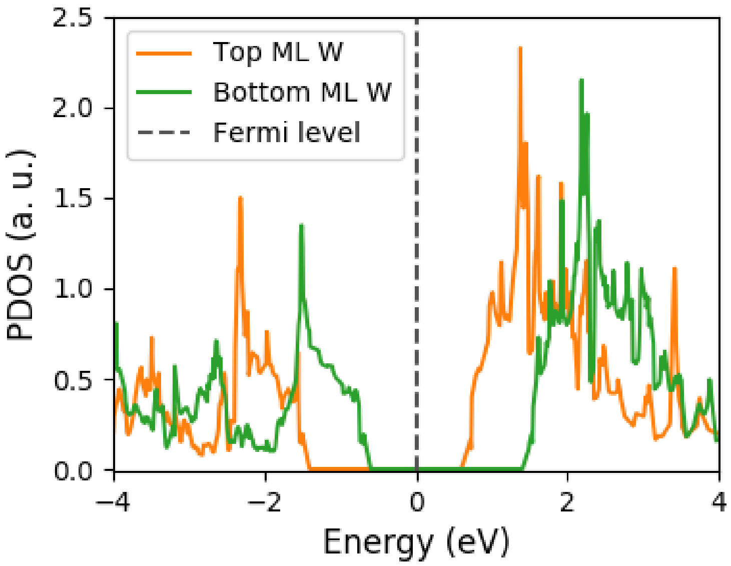


**Figure S11**: Desity of states projected onto the tungsten atoms in top and bottom MLs at $V_{TG}$=+$V$ and $V_{BG}$=-$V$. It can ve seen that each ML retains its ML bandgap, however the bandgap of overall BL is substantially narrower.
